# Supplementary material for: Retrieval-Augmented Embodied Agents
Source: arXiv:2404.11699 source file (2024-04-17)
Supplement: Supplementary file 1 [file X_suppl.tex]

\clearpage
\setcounter{page}{1}
\maketitlesupplementary
\section{Limitations}
Our research introduces retrieval-augmented embodied agents, equipping robots with access to an external policy memory bank to enhance policy learning. While our method has been evaluated in real-world environments and two simulated benchmarks, its performance in untested environments remains uncertain. Additionally, it's important to highlight that our real-world experiments were conducted using a Franka Emika Robot, and results may vary with different robotic systems. Our approach relies on Open X-Embodiment~\cite{padalkar2023openx}. Utilizing alternative external policy memory banks could lead to differing outcomes. The real-world environment we used is distinct from this project and is planned for release upon publication.

\section{More Experiments}
\subsection{Datasets}
In our simulation, we utilize two distinct datasets:
\begin{itemize}
    \item \textbf{Franka Kitchen}~\cite{fu2020d4rl} is focused on tasks such as sliding open the right door, opening a cabinet, turning on a light, adjusting the stovetop knob, and opening a microwave. Each demonstration includes 50 state-action pairs, making the demonstration length 50.
    \item \textbf{Meta-World}~\cite{yu2020metaworld} presents a challenging array of tasks requiring advanced object manipulation skills. These tasks include assembling a ring on a peg, picking and placing a block between bins, pushing a button, opening a drawer, and hammering a nail.
\end{itemize}

\subsection{Implementation Details}
In our retrieval module R, we use the off-the-shelf ImageBind~\cite{girdhar2023imagebind} model for both the query and memory encoders $E_{Q}$ and $E_{M}$. We use FAISS~\cite{faiss} to index the external memory M (Flat Index) and perform MIPS-based retrieval. For our policy generator G, we use a Transformer as depicted in the aforementioned section. We maximize take up to 3 policies. At inference time, we also retrieve and add $1 < K <= 3$ policies. The model is trained on A100 80G GPUs, implemented in PyTorch~\cite{paszke2019pytorch}. For all experiments, we use behavior cloning with mean squared loss as the optimization objective. The Franka-Kitchen is trained for 40K steps, while Maniskill-2 is trained for 20K steps. We use weight decay of 1e-6, cosine learning rate scheduler with warmup steps of 5\% total steps. The gradient clip is also applied. We use Adam optimizer with initial learning of 1e-3 and 3e-4 for Franka Kitchen and Maniskill-2, respectively. For the policy generator in simulated environments, we use five blocks, while in real-world experiments, we use 3 Transformer blocks.

\begin{table}[t]

\caption{Ablation study on in-context learning ability in terms of manipulation on novel objects.}
\centering
\resizebox{0.45\textwidth}{!}{\begin{tabular}{l|l|c}
\toprule
Methods & Objects & Success Rate\\ 
\midrule
\multirow{1}{*}{RAEA} & Unseen & 27 \\
Without policy memory bank & Unseen & 6\\
\bottomrule
\end{tabular}}
\label{table:unseen_object}
\end{table}
\begin{table}[t]

\caption{Ablation study on in-context learning ability in terms of manipulation on few-shot tasks.}
\centering
\resizebox{0.45\textwidth}{!}{\begin{tabular}{l|l|c}
\toprule
Methods & Training & Success Rate\\ 
\midrule
\multirow{1}{*}{RAEA} & Few-shot  & 18 \\
Without policy memory bank & Few-shot & 2\\
\bottomrule
\end{tabular}}
\label{table:few-shot_task}
\end{table}
\subsection{Ablation Study}
This section includes more experiments.
\\
\\
\noindent
\textit{In-context learning ability for RAEA: Novel object.} A primary advantage of the RAEA framework is its access to an external memory bank, potentially containing objects not included in the training datasets. We assessed RAEA's capability to manipulate objects unseen during training, viewing the retrieved policy as an in-context example for policy networks. Our experiments involved 10 objects not encountered during training, with each object undergoing 10 trials. The average success rate across all objects is documented in Table~\ref{table:unseen_object}. While performance did decrease when dealing with unseen objects compared to those encountered during training, it is noteworthy that our method, equipped with a policy memory bank, achieved a 21\% higher success rate than the baseline method that lacks this feature. This improvement is attributed to the baseline method’s sole reliance on instruction-observation mapping to identify novel objects, which can be challenging.
\\
\\
\noindent
\textit{In-context learning ability for RAEA: Few-shot tasks.} We also conducted an evaluation of our method on few-shot tasks, selecting five specific tasks trained with only five examples each. For each task, we executed ten trials and reported the average success rate across these five tasks. As observed in Table~\ref{table:few-shot_task}, utilizing the policy memory bank significantly enhances performance compared to not using it. We attribute this improvement to our in-context samples aiding the model in recognizing and executing these tasks effectively.
\\
\\
\noindent
\textit{Importance of Cross-Attention in Policy Generator.} A crucial element of our policy generator is the incorporation of cross-attention mechanisms to integrate instruction and observation data. We compared our method with FiLM~\cite{perez2018film}, a common technique for merging language and visual inputs, and also employed in RT1~\cite{brohan2022rt1}. We also examined the approach of directly concatenating input tokens. As indicated in Table~\ref{table:concat}, utilizing cross-attention resulted in a 7\% higher success rate compared to FiLM, and remarkably, its performance was 44\% superior to that achieved through direct concatenation of inputs.
\begin{table}[t]

\caption{Ablation study on cross-attention.}
\centering
\resizebox{0.3\textwidth}{!}{\begin{tabular}{l|c}
\toprule
Methods &  Success Rate\\ 
\midrule
Cross-Attention &  54 \\
FiLM~\cite{perez2018film} & 47\\
Direct concatenation & 10\\
\bottomrule
\end{tabular}}
\label{table:concat}
\end{table}
\\
\\
\noindent
\textit{Importance of Diversity in Policy Retriever.} 
As highlighted in \S3.2, maintaining diversity in the policy retriever is crucial for the effectiveness of our method. Specifically, we discard 70\% of the retrieved policies, which usually originate from similar trajectories. Our findings reveal that without dropping these similar tokens, the success rate plummets to 4\%. This significant decrease is largely attributed to the data structure commonly used in robotics, where datasets often comprise multiple frames. In most of these frames, the background remains static, leading to repetitive and uninformative data. This redundancy can impede the training process by overwhelming the model with non-essential information.
